# Supplementary material for: A Scalable Approach to Quantum Simulation via Projection-based Embedding
Source: arXiv:2203.01135 ancillary file (2022-05-17)
Supplement: Supplementary file 1 [file Supporting_Information.pdf]

# Supporting Information: A Scalable Approach to Quantum Simulation via Projection-based Embedding

Alexis Ralli,[*,†] Michael I. Williams de la Bastida,[*,†] and Peter V. Coveney[*,†,‡,¶]

†*Centre for Computational Science, Department of Chemistry, University College London, WC1H 0AJ, United Kingdom*

‡ *UCL Centre for Advanced Research Computing, Gower Street , London WC1E 6BT, United Kingdom*

¶ *Informatics Institute, University of Amsterdam, Amsterdam, 1098 XH, Netherlands*

E-mail: alexis.ralli.18@ucl.ac.uk; michael.williams.20@ucl.ac.uk; p.v.coveney@ucl.ac.uk

## Localisation

In this section, we describe how to generate a set of localized molecular orbitals (LMOs) from the cannoncial molecular orbitals of the global DFT calculation. This step is required in order to define each subsystem according to a certain metric discussed in further detail here.

We employ two methods to generate a set of localised molecular orbitals: the intrinsic bond orbitals (IBO)[1] and subsystem Projected AO DEcomposition (SPADE).[2] Other methods can be used, such as Pipek-Mezey (PM),[3] Foster-Boys (FB),[4] Edmiston-Ruedenberg (ER)[5] and fourth moment (FM) localization.[6]

## SPADE

SPADE is designed to localise electrons to the general region of an active site and environment.[7] This avoids the need for a threshold used to define the active and environment systems, as needed by the PM, FB, ER, FM and IBO approaches. The next section goes into more details about this.

We first restrict the $\mathbf{C}$ matrix to only the occupied molecular orbitals $\{\psi_{occ}\} \subset \{\psi\}$. As our aim is to localise electrons to one region; virtual orbitals need not be localised. The remaining MOs are made mutually orthogonal by rotation with the matrix defining the overlap of atomic orbitals $\mathbf{S}$:[7]

$$\bar{\mathbf{C}} = \mathbf{S}^{0.5}\mathbf{C}_{occ}. \tag{S.1}$$

We wish to find the relative contribution of the active region AOs to the occupied MOs, so we now restrict the matrix to only contributions from AOs associated to atoms in the active region $\bar{C}_A$. By making a singular value decomposition of this matrix:[7]

$$\bar{\mathbf{C}}_A = \mathbf{U}_A \mathbf{\Sigma}_A \mathbf{V}_A^{\star}, \tag{S.2}$$

we can determine a basis which localises the electrons of the active region. The column vectors of $\mathbf{V}_A$ are identical to the eigenvectors of $\bar{\mathbf{C}}_{occ}^{A\dagger}\bar{\mathbf{C}}_{occ}^{A}$.[7] A new set of orbitals are then obtained through a rotation of the original MOs $\mathbf{C}_{occ}$ as:

$$\mathbf{C}_{occ}^{SPADE} = \bar{\mathbf{C}}_{occ}\mathbf{V}_A, \tag{S.3}$$

where $\mathbf{C}_{occ}^{SPADE}$ are the SPADE orbitals. The singular values $\{\sigma\}$ of $\mathbf{\Sigma}_A$ allow appropriate partitioning of the orbital subspaces into active and environment subsystem.[7] The largest difference between successive singular values gives the partition of the SPADE MOs. Formally we write this as:

$$m_{occ}^{A} = \max_i\{\sigma_i - \sigma_{i+1}\}, \tag{S.4}$$

here $m_{occ}^{A}$ is the index $i$ where the largest difference occurs. The SPADE MOs (columns of $\mathbf{C}_{occ}^{SPADE}$) up to this index are the active MOs and the remaining orbitals (other columns of $\mathbf{C}_{occ}^{SPADE}$) are the environment orbitals.

## Intrinsic Bonding Orbitals

The intrinsic bonding orbitals (IBO) are generated from the canonical orbitals of a self-consistent field (SCF) calculation - in our case a Kohn-Sham density functional theory calculation.

Taking the canonical orbitals defined as:

$$|\psi_i\rangle = \sum_{j=1}^{K} \mathbf{C}_{ji} |\phi_j\rangle , \tag{S.5}$$

each MO $|\psi_i\rangle$ is hard to interpret, as each atomic orbital's (AO) basis functions $|\phi_j\rangle$ cannot be associated with a given atom. Normally MOs are highly delocalized and each $|\phi_j\rangle$ will contribute where it is needed most. Thus, we would like to expand the MOs over another minimal basis of free-atom AOs for each atom. This would make the wave function easy to interpret, but would be inaccurate and even incorrect, as free-atom AOs contain no polarization due to the molecular environment.

The approach by Knizia solves this issue by determining a set of polarized AOs $|\rho\rangle$, which are the intrinsic atomic orbitals (IAOs).[1] Summarising the main details, a free-atom basis is defined and the overlap with the basis used in the SCF calculation and itself is calculated. A projection is then performed to obtain the polarized AOs $|\rho\rangle$. These orbitals are orthogonalized to give an orthonormal minimal basis set consisting of the intrinsic atomic orbitals (IAOs).[1]

The utility of IAOs stems from the fact that they are directly associated with atoms, can be used to define atomic properties like partial charges and are basis set independent, unlike the Pipek-Mezey approach.

We can then localize the IAOs in a similar way to Pipek-Mezey. A Slater determinant $\left|\psi_{i'}^{LMO}\right\rangle = \sum_i^{occ} U_{ii'} \left|\psi_i\right\rangle$ is invariant to unitary rotations for occupied MOs $\left|\psi_i\right\rangle$. The intrinsic bonding orbitals (IBOs) are obtained by maximising[1]

$$L = \sum_{I}^{N_{atoms}} \sum_{i' \in occ} [n_I(i')]^4, \tag{S.6}$$

with respect to $U_{ii'}$. Here $n_I(i') = 2\sum_{\rho \in A} \langle \rho | i' \rangle \langle i' | \rho \rangle$, which is the number of $|i'\rangle$ electrons located on the IAOs $|\rho\rangle$ of atom $I$.[1]

In order to assign these localized molecular orbitals to the active and environment subsystems we calculate the percentage of the $i_{th}$ LMO over the active atoms as:

$$p_i^B = \frac{\sum_{\nu \in B} \mathbf{C}_{i\nu}^2}{\sum_{\nu=1}^{K} \mathbf{C}_{i\nu}^2}, \tag{S.7}$$

where $\nu \in B$ are the atomic orbital indices for the atoms defined in the active region. The denominator includes all the AOs of the $i_{th}$-th MO. This is the approach given in Equation 10 in the work of Koch *et al.*[8] Any $p_i^B > 95\%$ we associate to the active subsystem.

Our code on GitHub uses this metric for the other localization strategies supplied by PySCF. The code generates a localized $\mathbf{C}$ matrix, which can then be used in conjunction with Equation S.7.

## Embedded self-consistent field methodology

In this section we summarise how the embedded self-consistent field calculations are performed for the $\mu$-shift and Huzinaga methods. We consider restricted Hartree-Fock (RHF) calculations; extensions to the unrestricted case follow straightforwardly.

## $\mu$-shift RHF

To perform the $\mu$-shifted RHF calculation, only the core Hamiltonian is modified (Equation 13b), by adding $\mathbf{V}_{emb} + \mathbf{P}^{env}_{proj}$ to it. The $\mathbf{g}(\gamma^{act} + \gamma^{env})$ term is obtained from the global DFT calculation. The $\mathbf{g}(\gamma^{act})$ potential energy matrix is calculated in the same way, except the density matrix is set to be that of the active system only. The $\mu$-shift projector can then be defined using Equation 14.

The standard RHF algorithm can then be run, where the only difference is that the standard core Hamiltonian has been modified to be $\mathbf{h}_{emb}$.

## Huzinaga RHF

The Huzinaga RHF calculation is slightly more involved than the $\mu$-shifted method. At each self consistent field loop, when the new Fock matrix is defined, the Huzinaga projection operator $\mathbf{P}^{env}_{huz}$ must be built according to Equation 17. We reiterate this step uses the current Fock matrix in the self consistent field loop. The embedded Fock matrix is then constructed according to equation 12, where the potential energy matrix $\mathbf{V}^{proj}_{emb}$ (Equation 13a) is defined in the same manor as the $\mu$-shift RHF method. Given this embedded Fock matrix, $\mathbf{F}^{act}_{emb}\mathbf{C} = \mathbf{S}\mathbf{C}\epsilon$ can be solved via standard SCF approaches. This generates a set of new MO coefficients $\mathbf{C}$ that are used to construct the new Fock matrix. This process is repeated until the energy converges as usual in an SCF calculation.

# Active Atom Selection

As the number of active atoms is configurable with this method, we demonstrate the effect of altering this parameter using cyclopentane. Figure S.1 shows the change in calculated ground state energy, qubit count and number of terms in the Jordan-Wigner encoded qubit Hamiltonian.

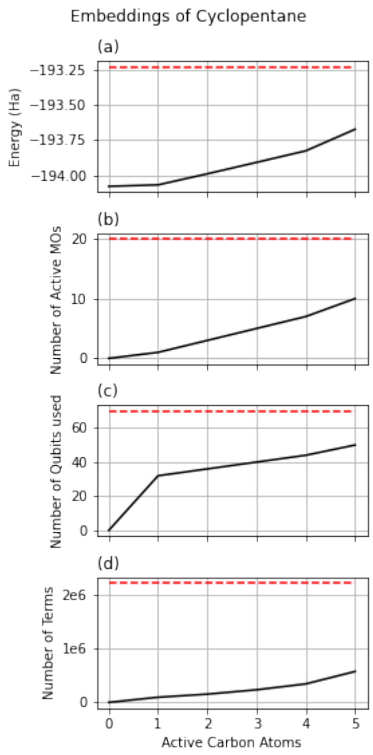


Figure S.1: Results of cyclopentane embedding, with increasing numbers of carbon atoms assigned to the active region. For each, IBO localisation was used; results for the $\mu$-shift and Huzinaga projector are overlapping and indistinguishable. Different methods do not give noticeably distinct results. (a) Ground state energy. (b) Number of occupied molecular orbitals assigned to the active region. (c) Number of qubits in output Hamiltonian. (d) Number of terms in the Jordan-Wigner encoded qubit Hamiltonian.

# Molecular Ground State Energy

Our method provides flexibility to select a localisation method. In addition to the result displayed in Figure 2, which were calculated using the SPADE projection method, we present results for the same molecules using the Intrinsic Bonding Orbitals localisation method in Figure S.2. Numerical values for these results are given in Table S.1 for reference values, and Tables S.2 and S.3 for our calculated results.

Table S.1: Full-system reference values for embedding calculations of small molecules, as shown in Figures 2 and S.2. $\epsilon_{DFT}$ gives the difference between full-system RKS DFT, using the B3LYP functional, and CCSD(T). $Q$ and $|H|$ give respectively the number of qubits and terms in the Jordan-Wigner encoded qubit Hamiltonian of the full system.

| Molecule | $\epsilon_{DFT}$ | $Q$ | $\|H\|$ |
|---|---|---|---|
| N-methylmethanamine | 0.5733 | 44 | 338971 |
| acetaldehyde | 0.569 | 38 | 182702 |
| acetonitrile | 0.485 | 36 | 136067 |
| ethanamine | 0.573 | 44 | 329283 |
| ethanol | 0.609 | 42 | 283020 |
| fluoroethane | 0.637 | 40 | 217385 |
| formamide | 0.619 | 36 | 138235 |

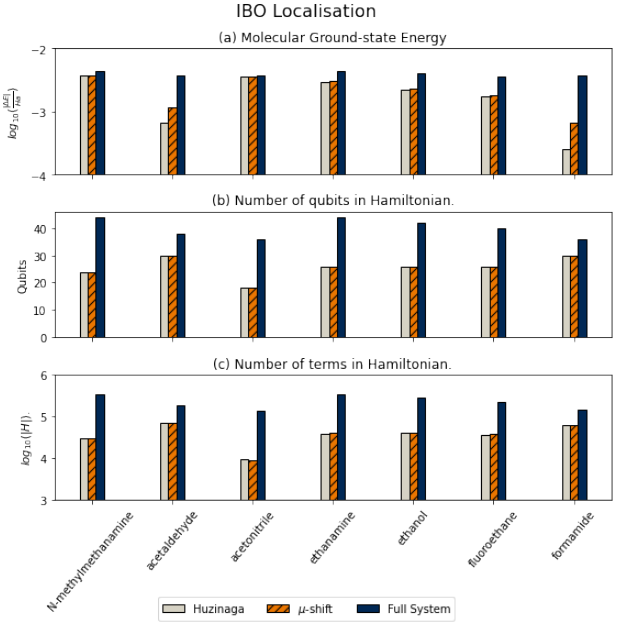


Figure S.2: Results for embedding of small molecules using the IBO localisation method. (a) Ground state energies for small molecules, with full-system DFT energy as reference, $\mu$-shift CCSD embedding energy in orange and Huzinaga CCSD embedding in grey. All values are given as a difference from whole system CCSD(T) energy. (b) The number of qubits required to describe the embedded Hamiltonian, with reference showing the number required for the full system Hamiltonian. (c) The number of terms in the Jordan-Wigner encoded qubit Hamiltonian for each molecule. Again the reference gives the number needed for the full system Hamiltonian.

# Strong Correlation

We provide the numerical details of our strongly correlated $H_2O$ simulation in this section.

These results form Figure 3 in the main text.

Table S.2: Numerical values of the calculations shown in Figure S.2. For each calculation the energy difference between CCSD(T)-in-DFT embedding and full system CCSD(T), $\epsilon$, is given. The number of qubits $Q$ and number of terms in the output Jordan-Wigner encoded qubit Hamiltonian $|H|$ are given. Results for IBO localisation are shown, with results for SPADE in Table S.3 reference values using the full system given in Table S.1

| Molecule | $\epsilon_{Huz}$ | $\epsilon_{\mu}$ | $Q_{Huz}$ | $Q_{\mu}$ | $\lvert H_{emb}^{Huz}\rvert$ | $\lvert H_{emb}^{\mu}\rvert$ |
|---|---|---|---|---|---|---|
| N-methylmethanamine | 0.491 | 0.494 | 24 | 24 | 29701 | 29737 |
| acetaldehyde | 0.099 | 0.178 | 30 | 30 | 70118 | 69554 |
| acetonitrile | 0.462 | 0.462 | 18 | 18 | 9232 | 9016 |
| ethanamine | 0.394 | 0.399 | 26 | 26 | 38716 | 39924 |
| ethanol | 0.340 | 0.350 | 26 | 26 | 40948 | 41060 |
| fluoroethane | 0.299 | 0.312 | 26 | 26 | 35020 | 38180 |
| formamide | 0.043 | 0.109 | 30 | 30 | 62434 | 61914 |

Table S.3: Numerical values of the calculations shown in Figure 2. For each calculation the energy difference between CCSD(T)-in-DFT embedding and full system CCSD(T), $\epsilon$, is given. The number of qubits $Q$ and number of terms in the output Jordan-Wigner encoded qubit Hamiltonian $|H|$ are given. Results for SPADE localisation are shown, with results for IBO in Table S.2 reference values using the full system given in Table S.1

| Molecule | $\epsilon_{Huz}$ | $\epsilon_{\mu}$ | $Q_{Huz}$ | $Q_{\mu}$ | $\lvert H_{emb}^{Huz}\rvert$ | $\lvert H_{emb}^{\mu}\rvert$ |
|---|---|---|---|---|---|---|
| N-methylmethanamine | 0.135 | 0.169 | 36 | 36 | 152223 | 152415 |
| acetaldehyde | 0.098 | 0.176 | 30 | 30 | 70474 | 69982 |
| acetonitrile | 0.403 | 0.409 | 20 | 20 | 13439 | 13111 |
| ethanamine | 0.136 | 0.169 | 36 | 36 | 145067 | 149819 |
| ethanol | 0.132 | 0.169 | 34 | 34 | 120928 | 121036 |
| fluoroethane | 0.136 | 0.170 | 32 | 32 | 85781 | 89377 |
| formamide | 0.045 | 0.110 | 30 | 30 | 62366 | 61958 |

We performed projection based embedding calculations, at different molecular geometries, for two different active regions. One has the atoms in the fixed OH bond set active and the other has the atoms in the changing OH bond set active. The structure for $H_2O$ with an OH bond length of 0.4 $Å$ is given in Table S.4. The other geometries can be generated from this structure. Tables S.5 and S.6 summarise the numerical results for the different active systems.

Table S.4: Cartesian coordinates of atoms in $H_2O$ for the structure with an OH bond length of 0.4 $Å$ defined from the first H and O atoms in this Table. The other structures (different OH bond lengths) were generated from this file by changing the position of the first H atom. Note the H-O-H angle remained fixed.

| atom | x | y | z |
|---|---|---|---|
| H | 0.3751747 | 0.0000000 | 0.1387225 |
| O | 0.0000000 | 0.0000000 | 0.0000000 |
| H | -0.7493682 | 0.0000000 | 0.2770822 |

Table S.5: Numerical values of the calculations shown in Figure 3 for the case when the changing OH bond is set as the active region. For each calculation the energy error is reported as the absolute difference between FCI energy and the embedded calculation (where embedded Hamiltonian has been diagonalized to give the exact ground state). The number of qubits $Q$ and number of terms in the output Jordan-Wigner encoded qubit Hamiltonian $|H|$ are given.

| OH length | $\epsilon_{DFT}$ | $\epsilon_{Huz}$ | $\epsilon_{\mu}$ | $\|H_{full}\|$ | $\|H_{emb}^{Huz}\|$ | $\|H_{emb}^{\mu}\|$ | $Q_{full}$ | $Q_{Huz}$ | $Q_{\mu}$ | # active MOs |
|---|---|---|---|---|---|---|---|---|---|---|
| 0.400000 | 0.278880 | 0.006952 | 0.006953 | 2110 | 1079 | 1079 | 14 | 12 | 12 | 4 |
| 0.600000 | 0.274200 | 0.009325 | 0.009326 | 2110 | 1079 | 1079 | 14 | 12 | 12 | 4 |
| 0.798954 | 0.270965 | 0.012913 | 0.012914 | 1086 | 1079 | 1079 | 14 | 12 | 12 | 4 |
| 1.000000 | 0.269410 | 0.017567 | 0.017568 | 2110 | 1079 | 1079 | 14 | 12 | 12 | 4 |
| 1.200000 | 0.266920 | 0.023415 | 0.023415 | 2110 | 1079 | 1079 | 14 | 12 | 12 | 4 |
| 1.500000 | 0.249844 | 0.033200 | 0.033200 | 2110 | 1079 | 1079 | 14 | 12 | 12 | 4 |
| 2.000000 | 0.186272 | 0.040638 | 0.040639 | 2110 | 1079 | 1079 | 14 | 12 | 12 | 4 |
| 3.000000 | 0.118887 | 0.048521 | 0.048522 | 2342 | 1543 | 1551 | 14 | 12 | 12 | 4 |
| 4.000000 | 0.102433 | 0.048525 | 0.048525 | 2526 | 1819 | 1819 | 14 | 12 | 12 | 4 |
| 5.000000 | 0.100664 | 0.048552 | 0.048553 | 3054 | 1795 | 1795 | 14 | 12 | 12 | 4 |

Table S.6: Numerical values of the calculations shown in Figure 3 for the case when the fixed OH bond is set as the active region. For each calculation the energy error is reported as the absolute difference between FCI energy and the embedded calculation (where embedded Hamiltonian has been diagonalized to give the exact ground state). The number of qubits $Q$ and number of terms in the output Jordan-Wigner encoded qubit Hamiltonian $|H|$ are given.

| OH length | $\epsilon_{DFT}$ | $\epsilon_{Huz}$ | $\epsilon_{\mu}$ | $\|H_{full}\|$ | $\|H_{emb}^{Huz}\|$ | $\|H_{emb}^{\mu}\|$ | $Q_{full}$ | $Q_{Huz}$ | $Q_{\mu}$ | # active MOs |
|---|---|---|---|---|---|---|---|---|---|---|
| 0.400000 | 0.278880 | 0.093234 | 0.093229 | 2110 | 1079 | 1079 | 14 | 12 | 12 | 4 |
| 0.600000 | 0.274200 | 0.025531 | 0.025529 | 2110 | 1079 | 1079 | 14 | 12 | 12 | 4 |
| 0.798954 | 0.270965 | 0.012913 | 0.012914 | 1086 | 1079 | 1079 | 14 | 12 | 12 | 4 |
| 1.000000 | 0.269410 | 0.035443 | 0.035443 | 2110 | 1079 | 1079 | 14 | 12 | 12 | 4 |
| 1.200000 | 0.266920 | 0.046838 | 0.046838 | 2110 | 1079 | 1079 | 14 | 12 | 12 | 4 |
| 1.500000 | 0.249844 | 0.039789 | 0.039789 | 2110 | 1079 | 1079 | 14 | 12 | 12 | 4 |
| 2.000000 | 0.186272 | 0.020758 | 0.020758 | 2110 | 1079 | 1079 | 14 | 12 | 12 | 4 |
| 3.000000 | 0.118887 | 0.087767 | 0.087767 | 2210 | 1079 | 1083 | 14 | 12 | 12 | 4 |
| 4.000000 | 0.101794 | 0.099082 | 0.099082 | 2294 | 1655 | 1663 | 14 | 12 | 12 | 4 |
| 5.000000 | 0.100663 | 0.106092 | 0.106092 | 3054 | 1783 | 1799 | 14 | 12 | 12 | 4 |

# References

(1) Knizia, G. Intrinsic Atomic Orbitals: An Unbiased Bridge between Quantum Theory and Chemical Concepts. *Journal of Chemical Theory and Computation* **2013**, *9*, 4834–4843.

(2) Manby, F. R.; Stella, M.; Goodpaster, J. D.; Miller, T. F. A Simple, Exact Density-Functional-Theory Embedding Scheme. *Journal of Chemical Theory and Computation* **2012**, *8*, 2564–2568, PMID: 22904692.

(3) Pipek, J.; Mezey, P. G. A fast intrinsic localization procedure applicable for ab initio and semi-empirical linear combination of atomic orbital wave functions. *Journal of Chemical Physics* **1989**, *90*, 4916–4926.

(4) Foster, J.; Boys, S. Canonical configurational interaction procedure. *Reviews of Modern Physics* **1960**, *32*, 300.

(5) Edmiston, C.; Ruedenberg, K. Localized atomic and molecular orbitals. *Reviews of Modern Physics* **1963**, *35*, 457.

(6) Høyvik, I.-M.; Jansik, B.; Jørgensen, P. Orbital localization using fourth central moment minimization. *Journal of Chemical Physics* **2012**, *137*, 224114.

(7) Claudino, D.; Mayhall, N. J. Automatic Partition of Orbital Spaces Based on Singular Value Decomposition in the Context of Embedding Theories. *Journal of Chemical Theory and Computation* **2019**,

(8) Giovannini, T.; Koch, H. Energy-based molecular orbital localization in a specific spatial region. *Journal of Chemical Theory and Computation* **2020**, *17*, 139–150.
